# Supplementary material for: Distinguishing Legendrian knots of topological type $7_4$, $9_{48}$ and $10_{136}$
Source: arXiv:2306.15461 ancillary file (2024-01-30)

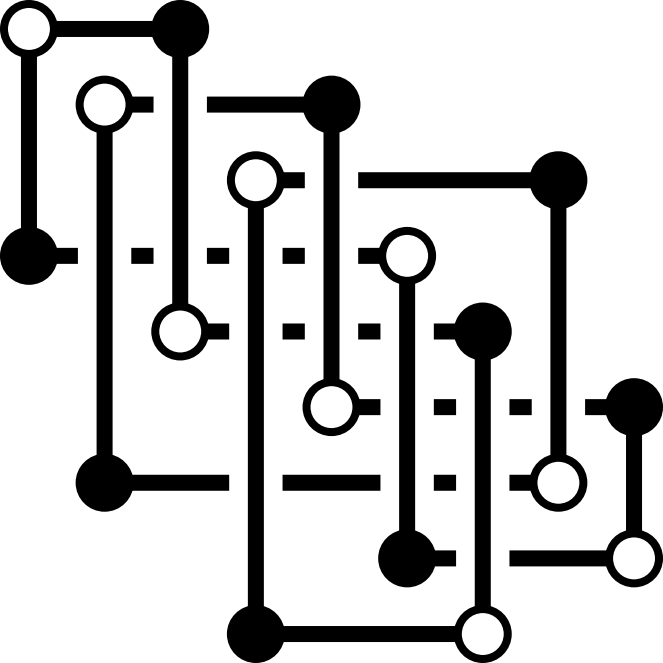

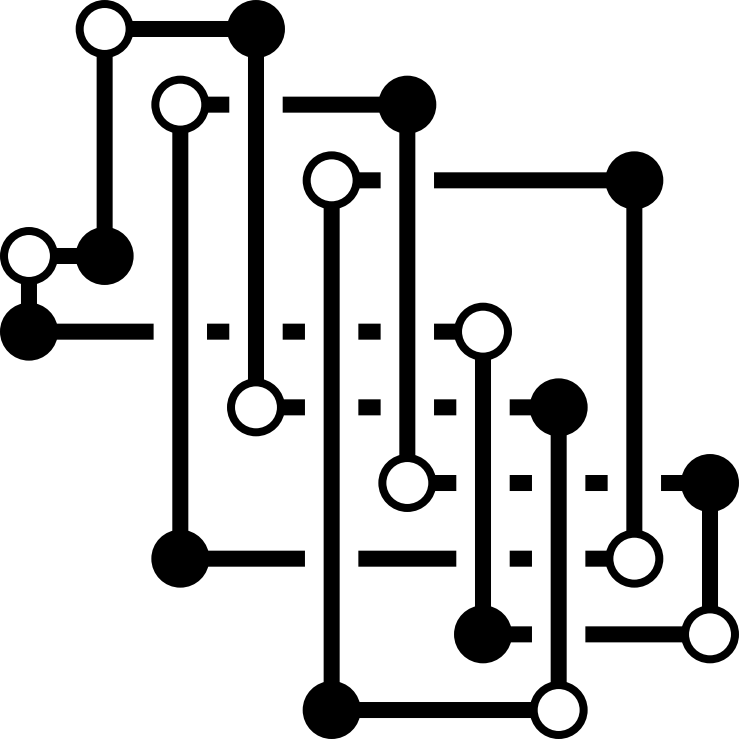

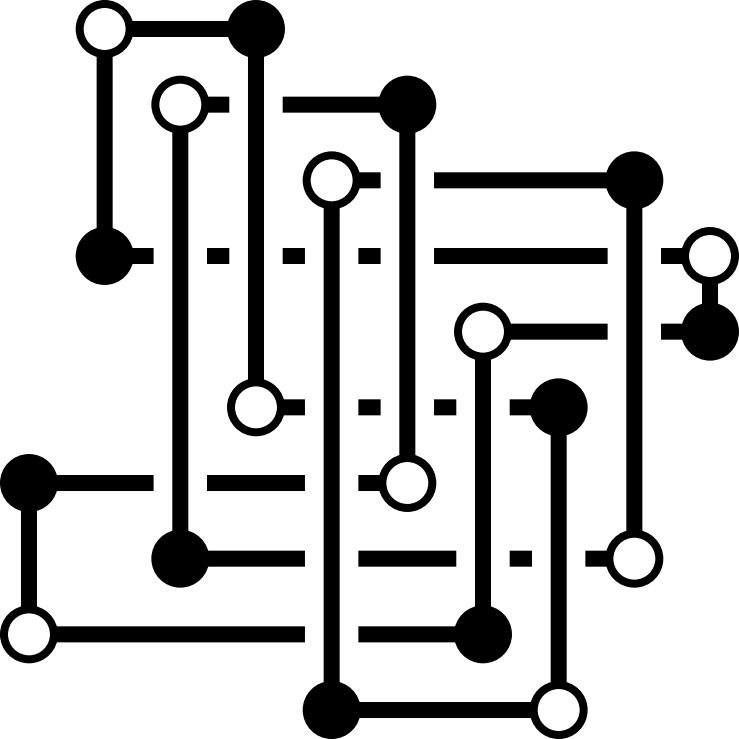

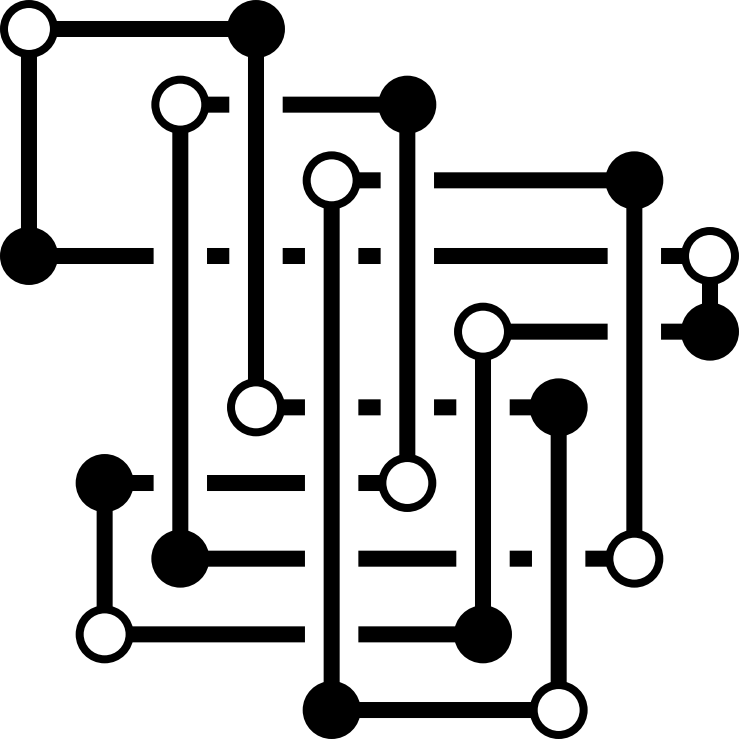

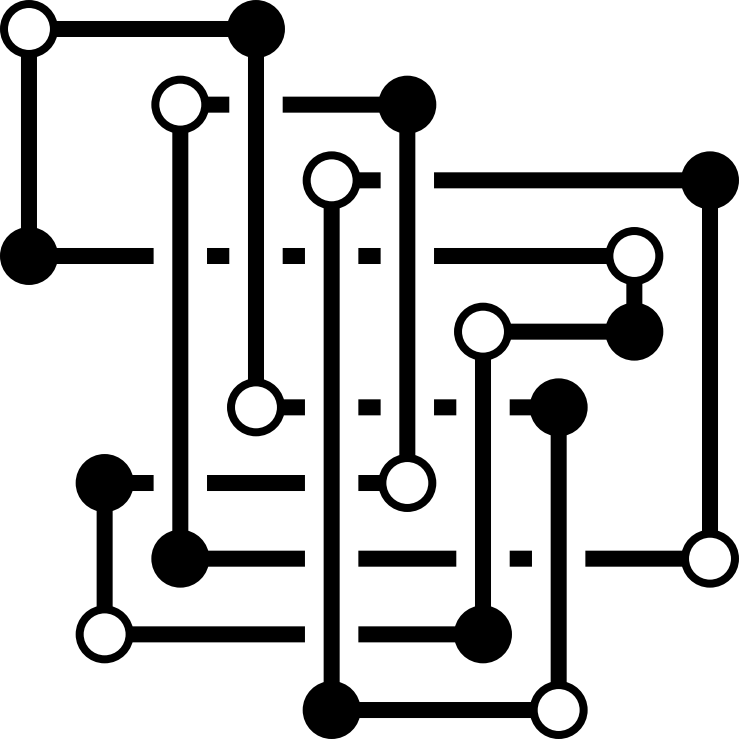

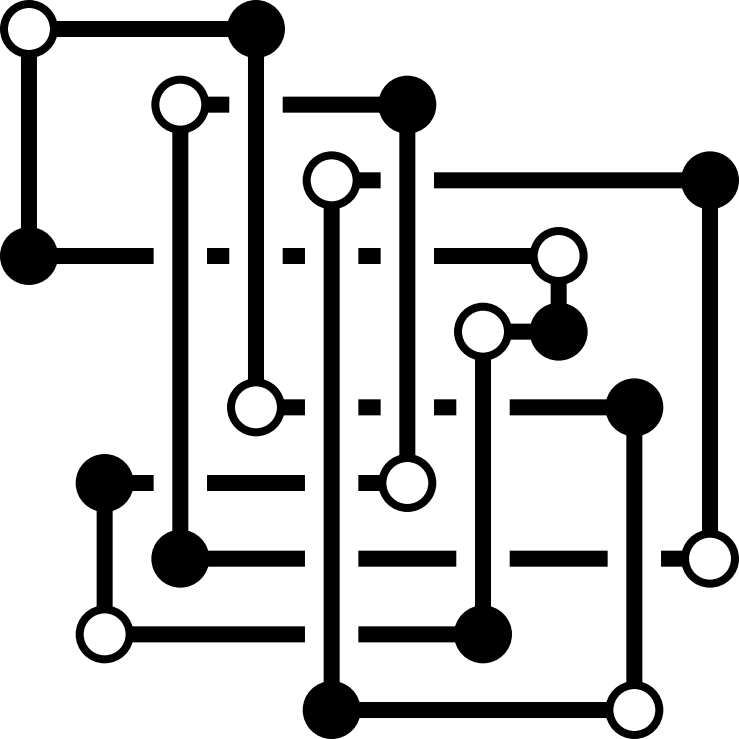

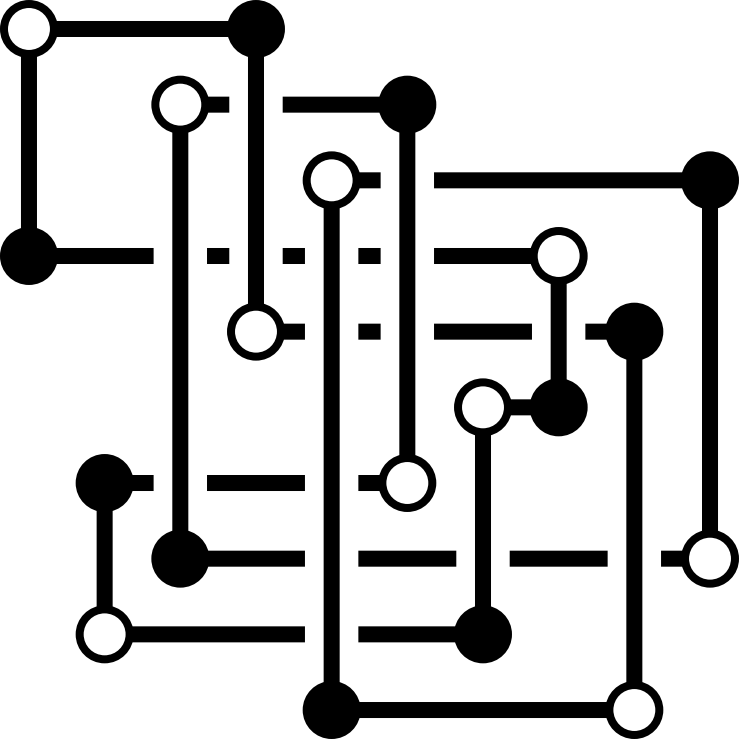

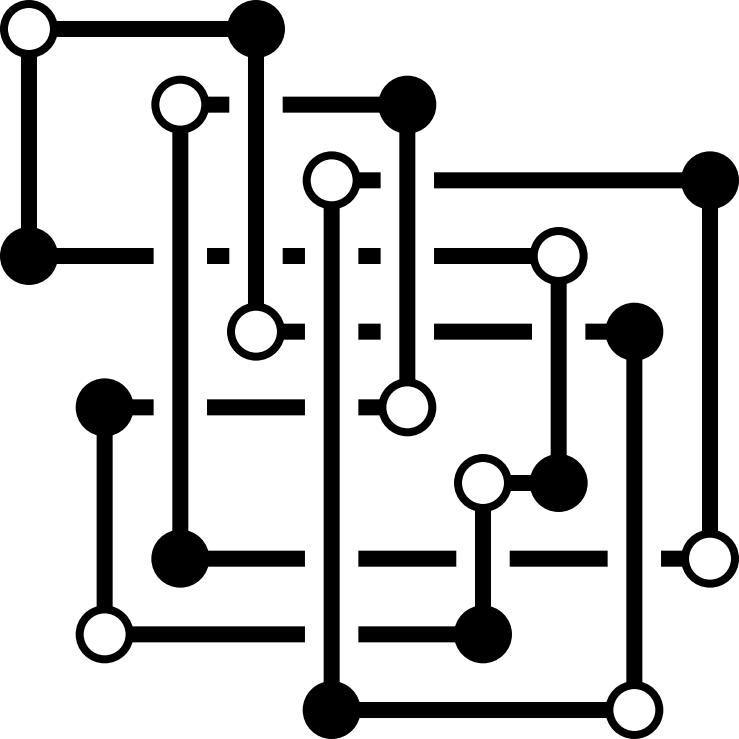



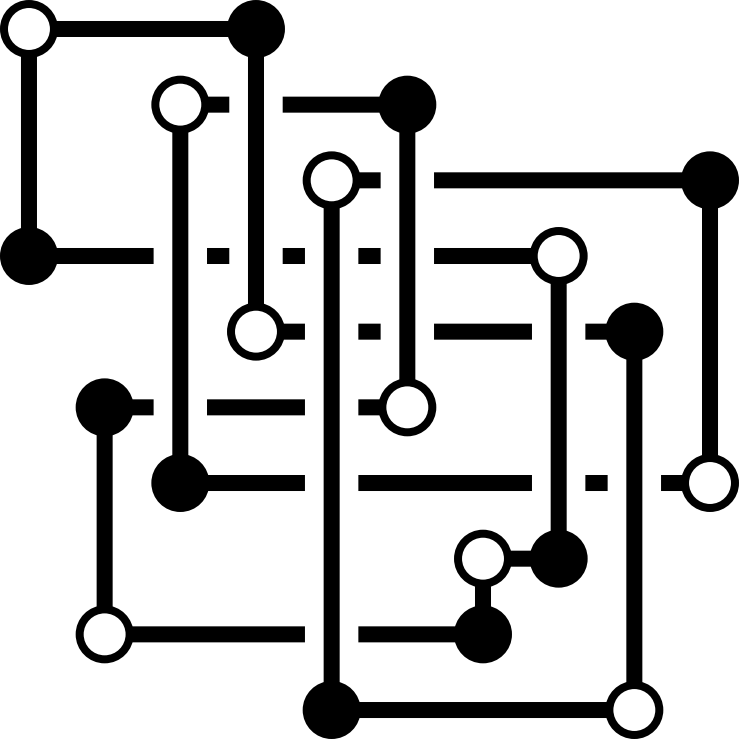

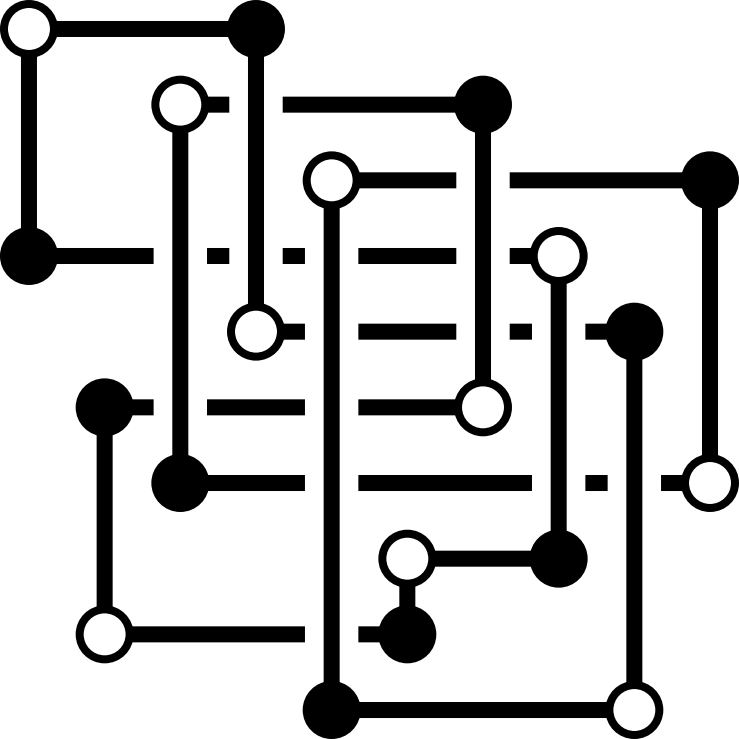

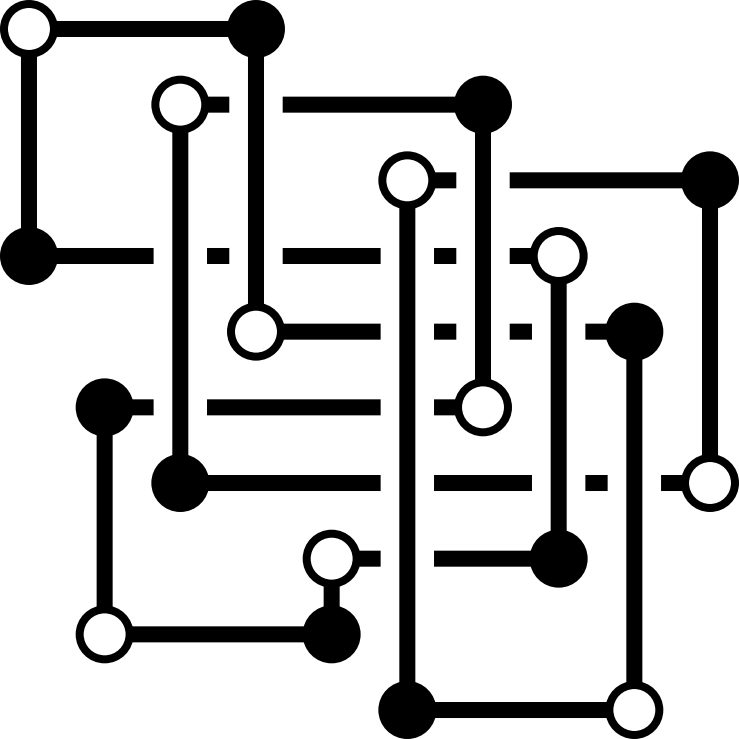

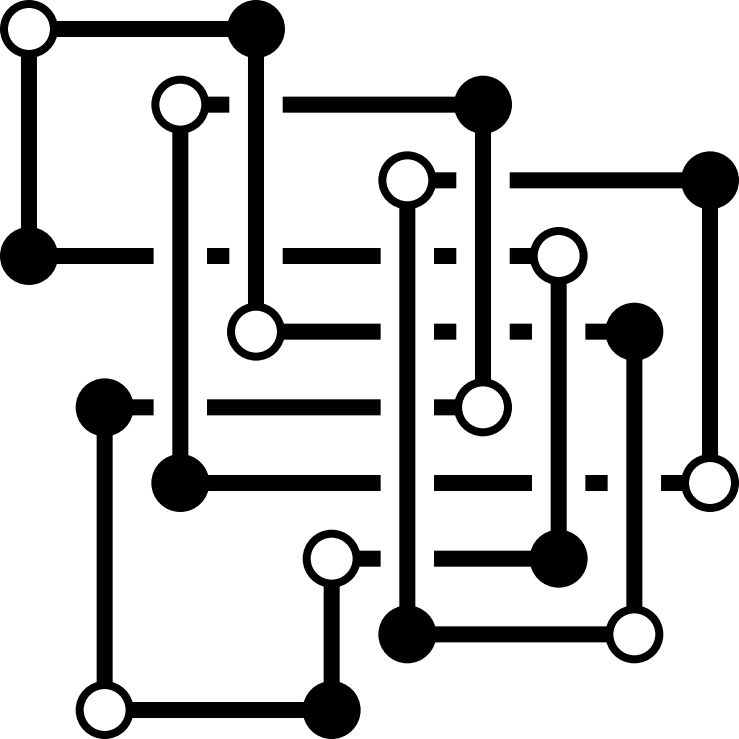

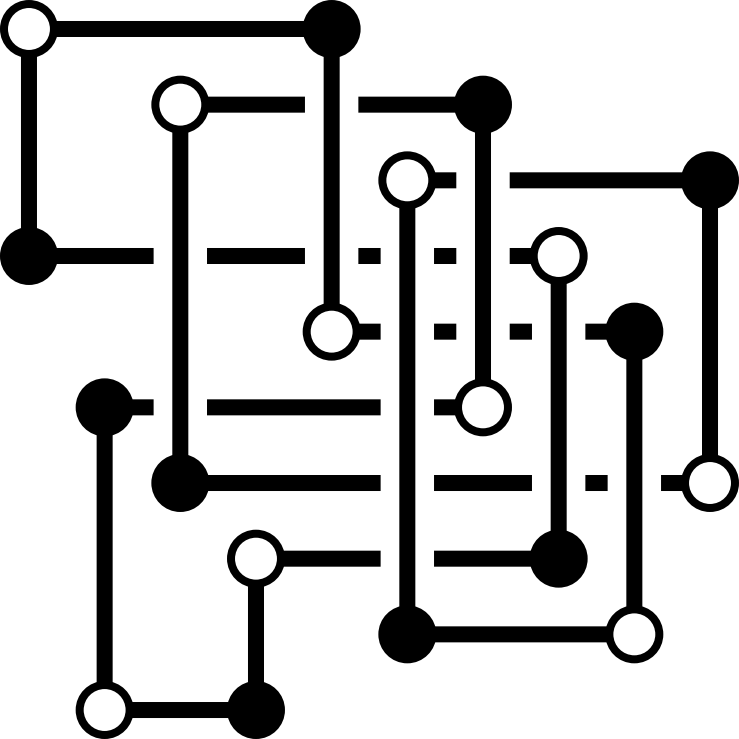

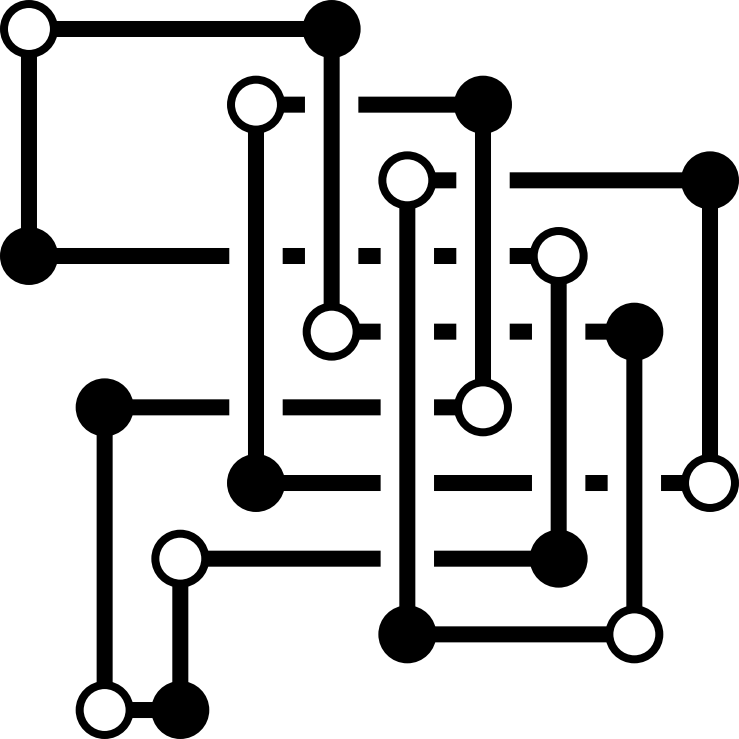

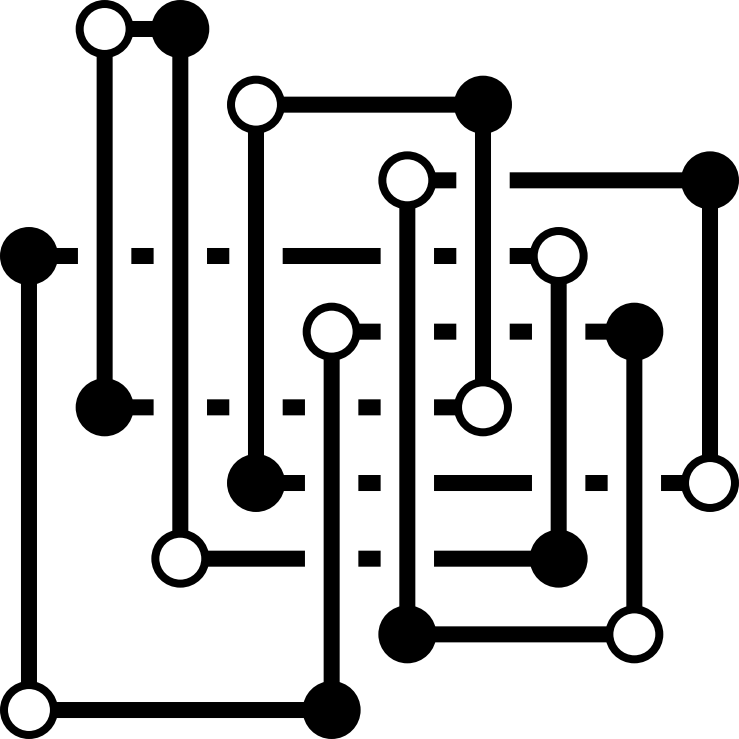

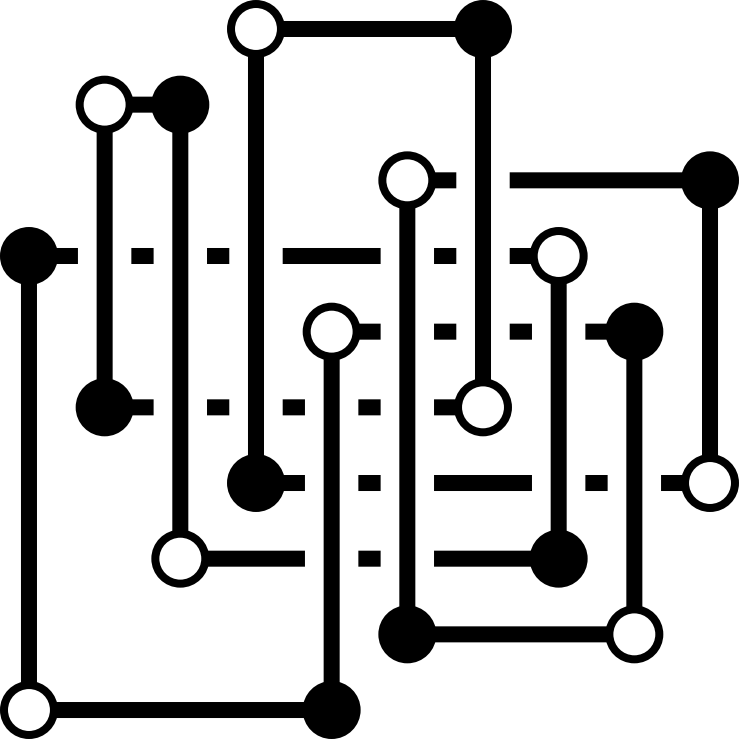



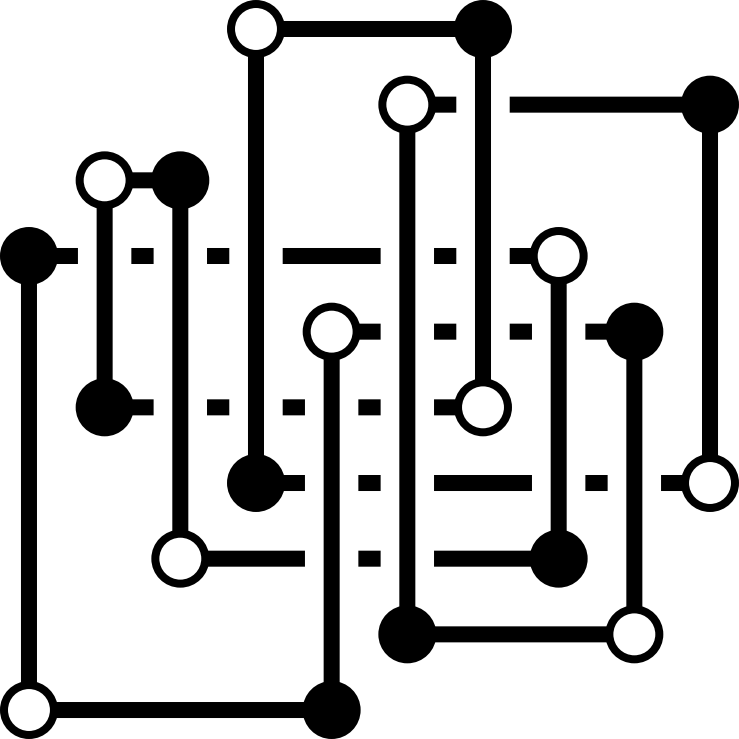

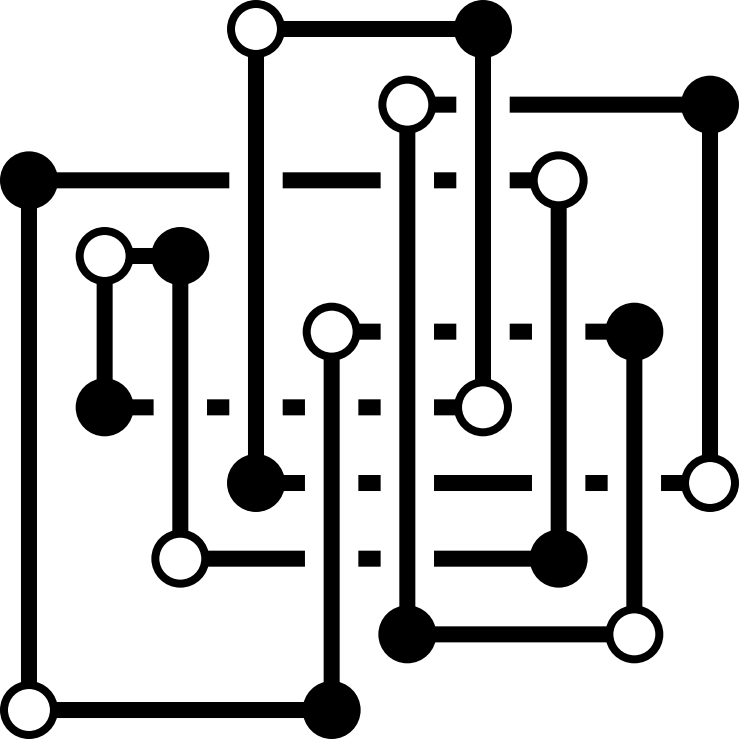

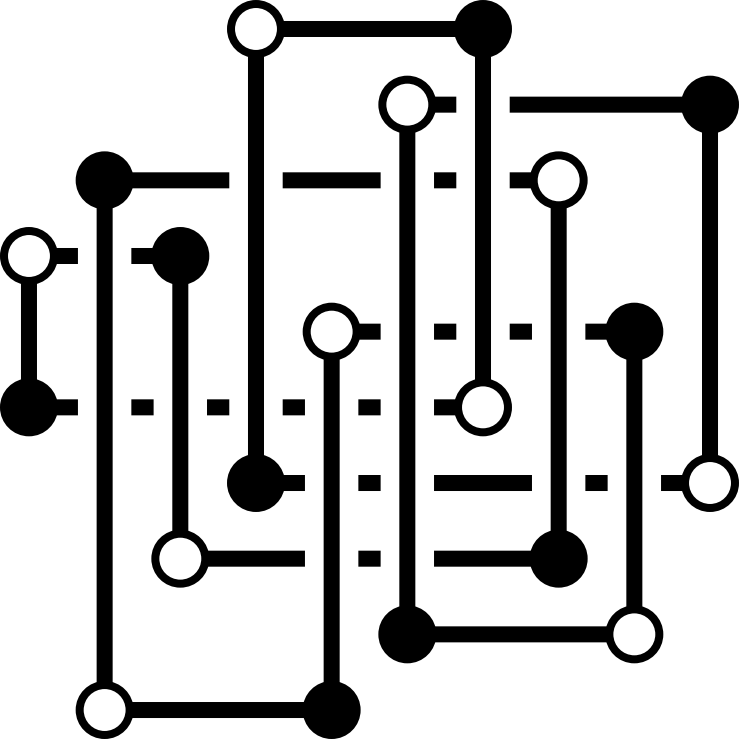

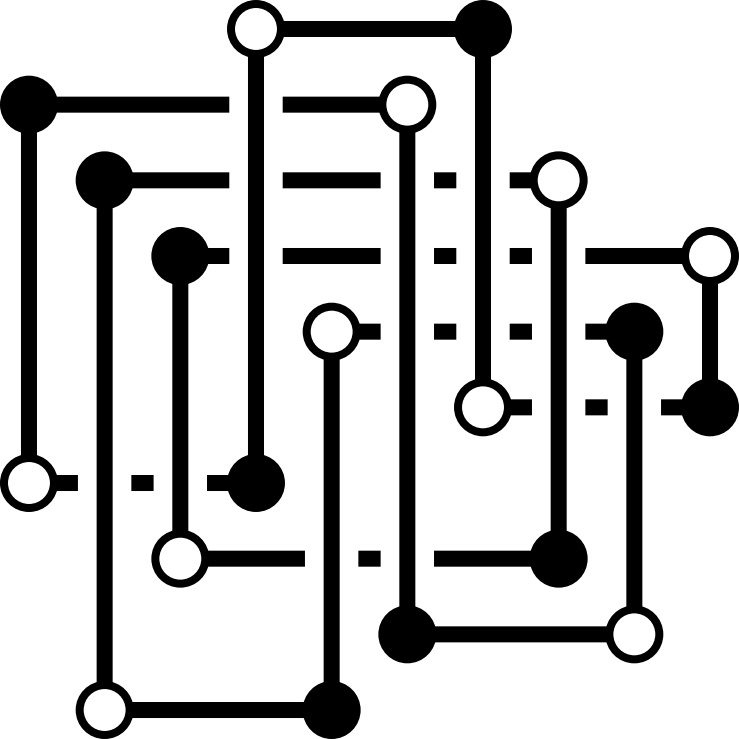

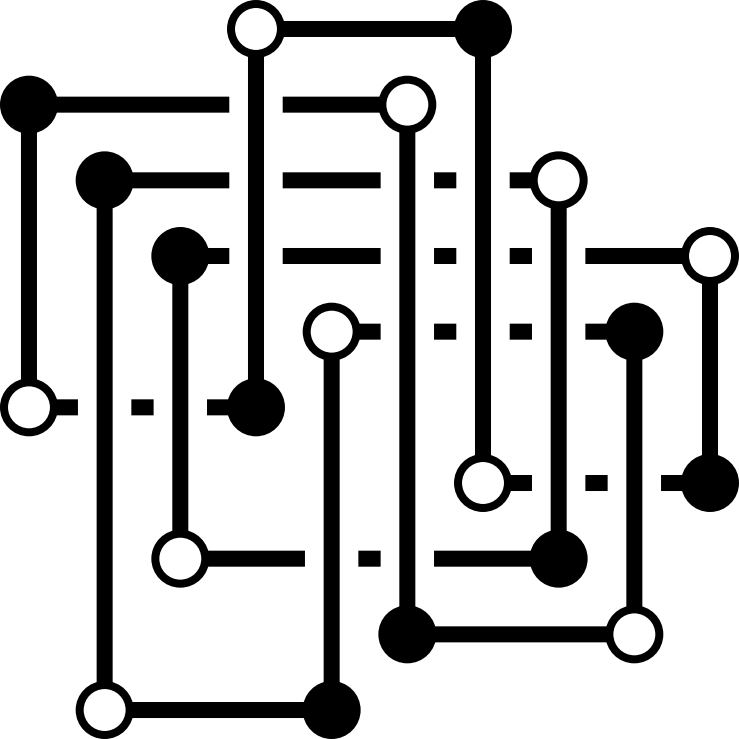

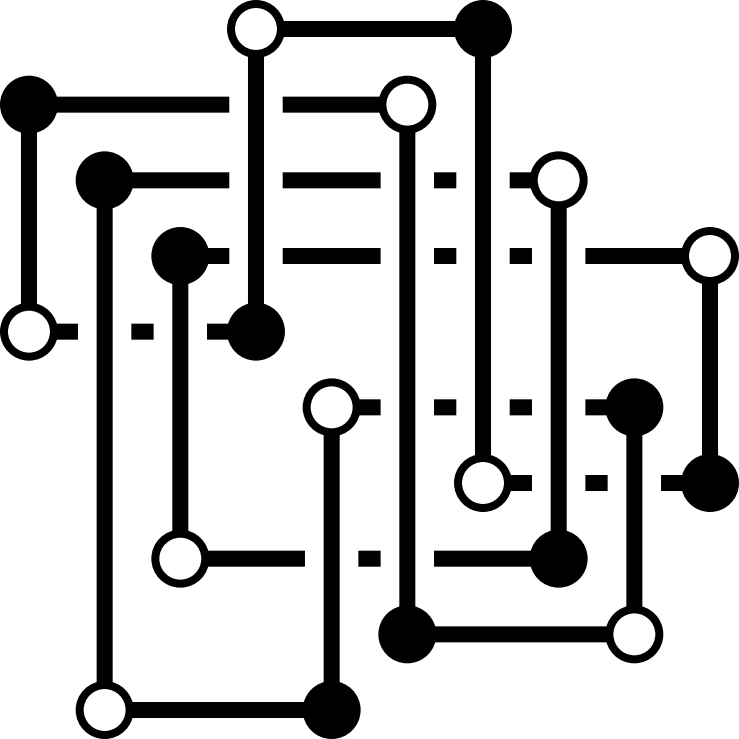

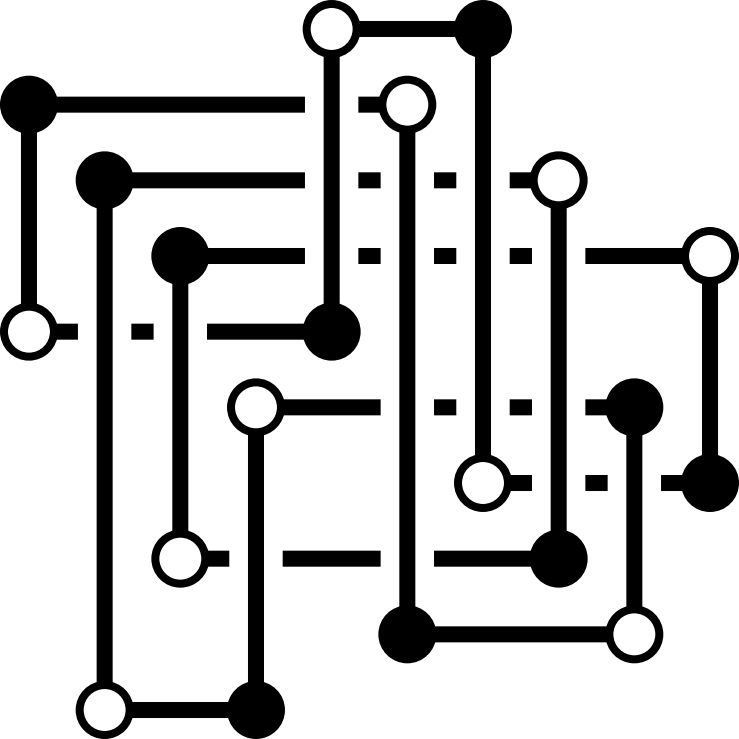

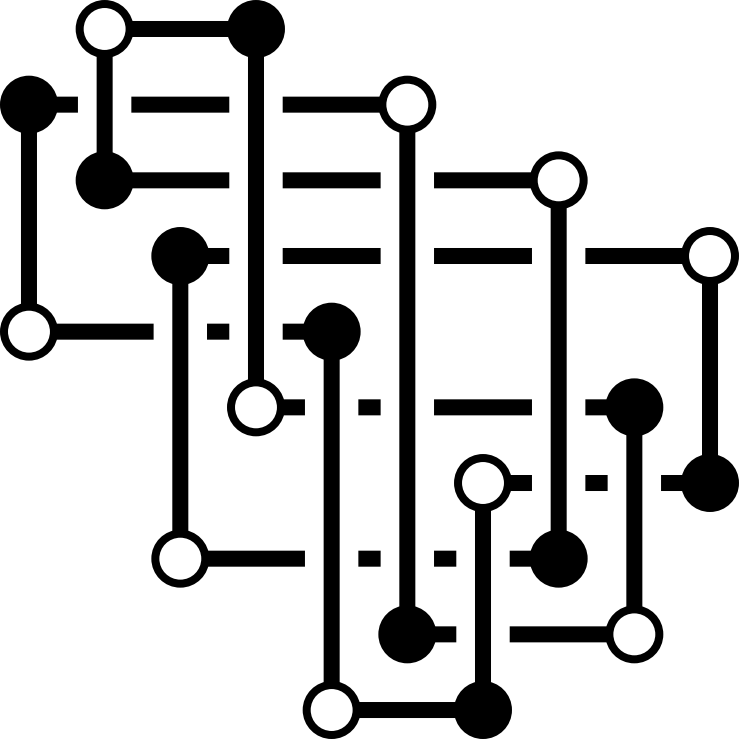



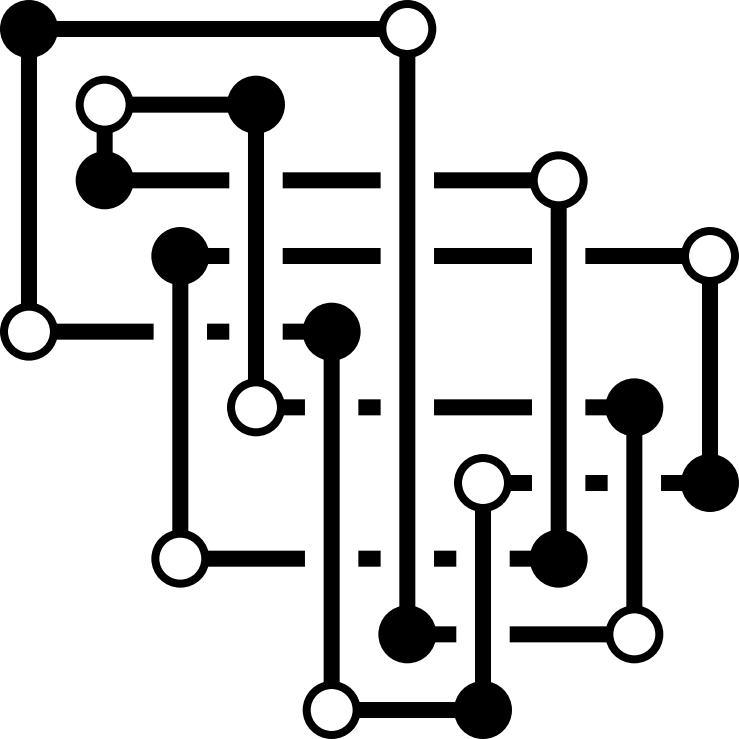

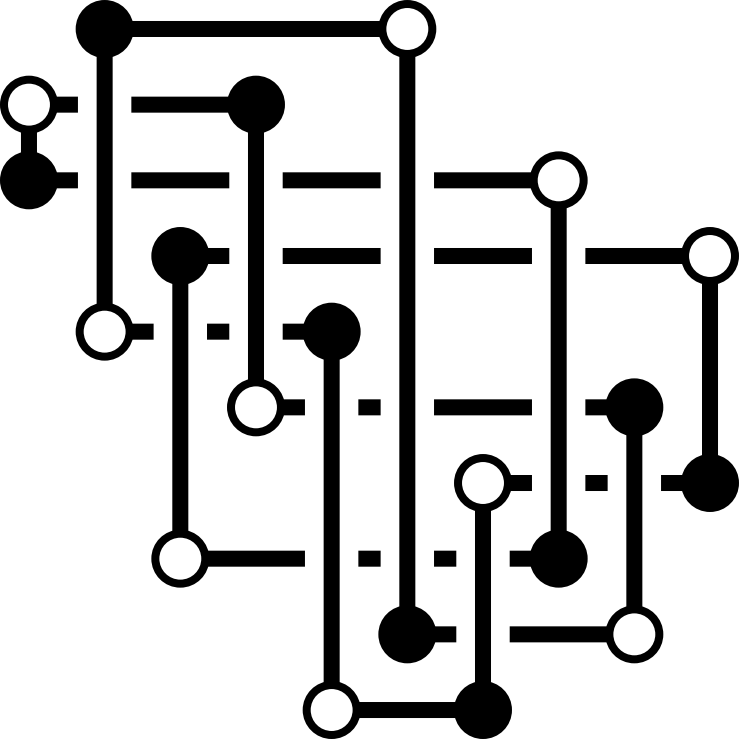

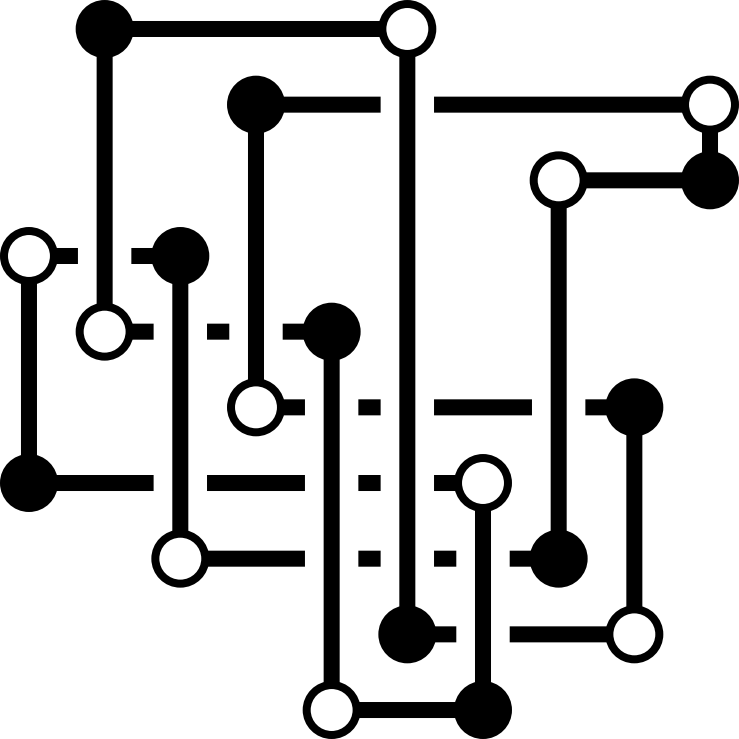

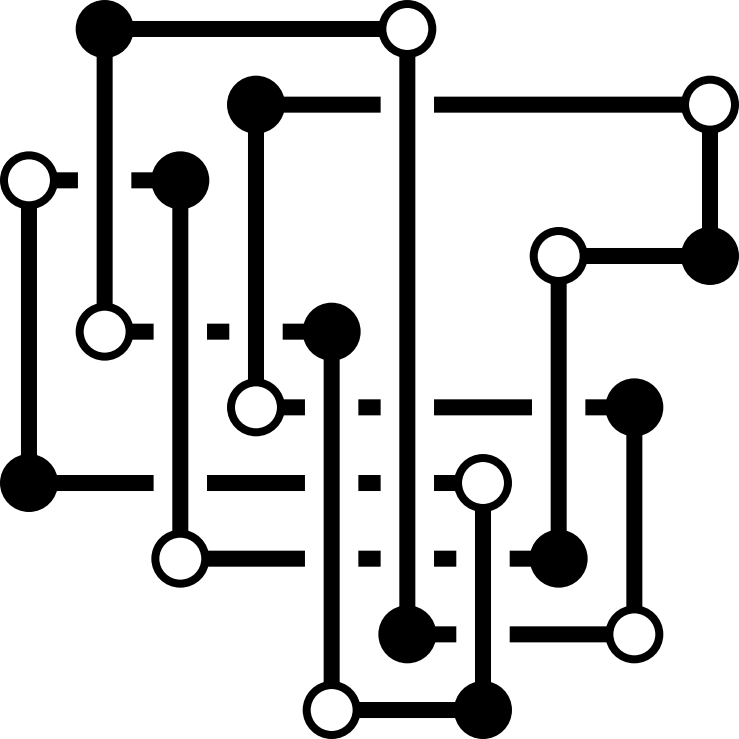

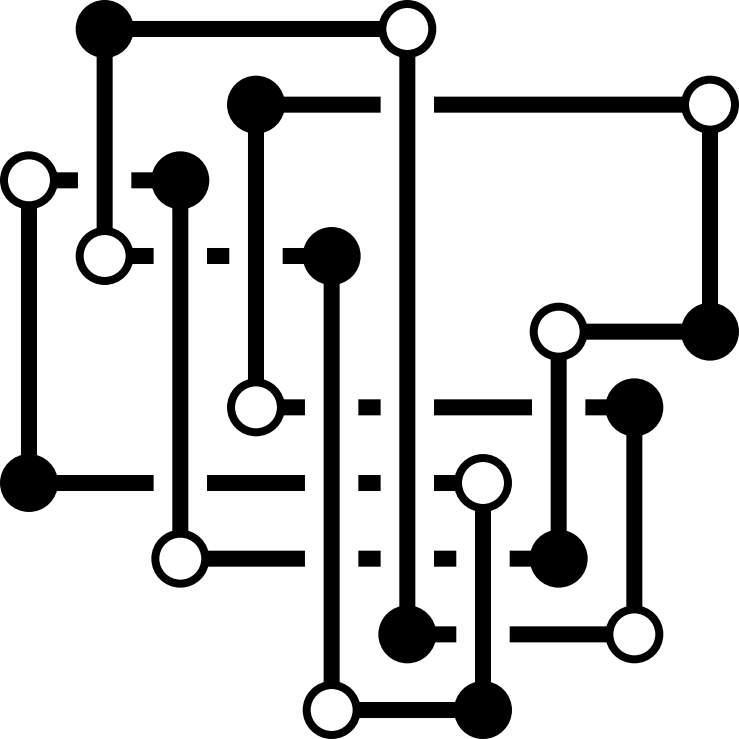

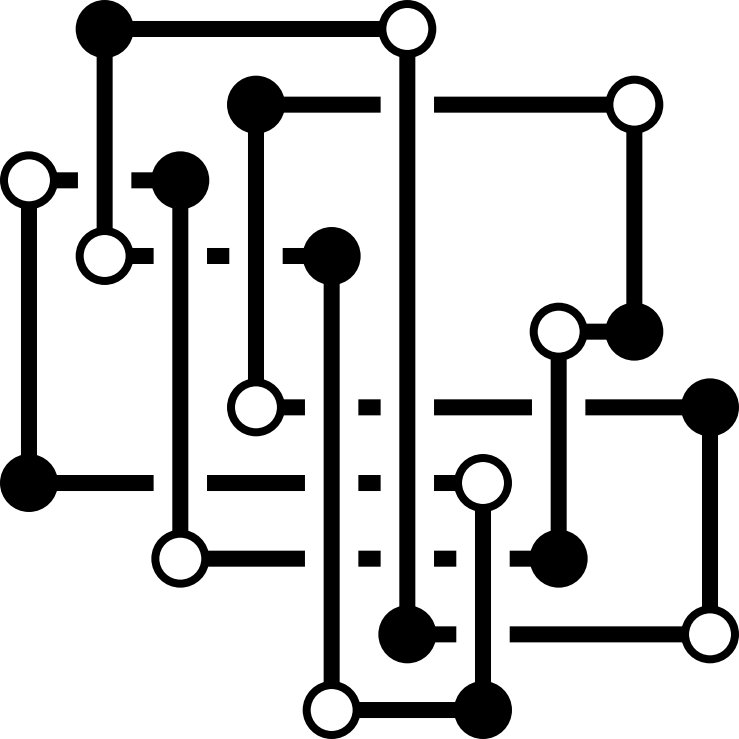

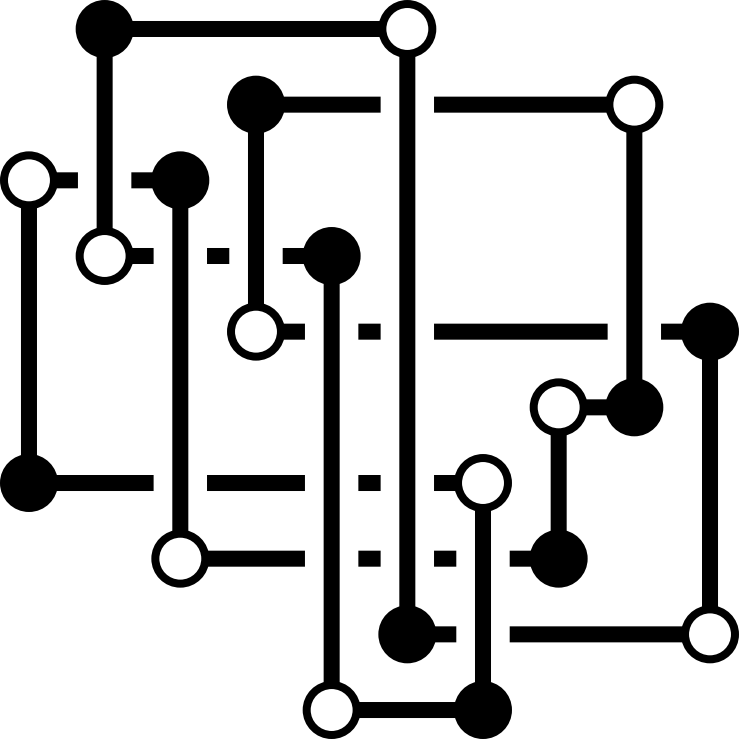

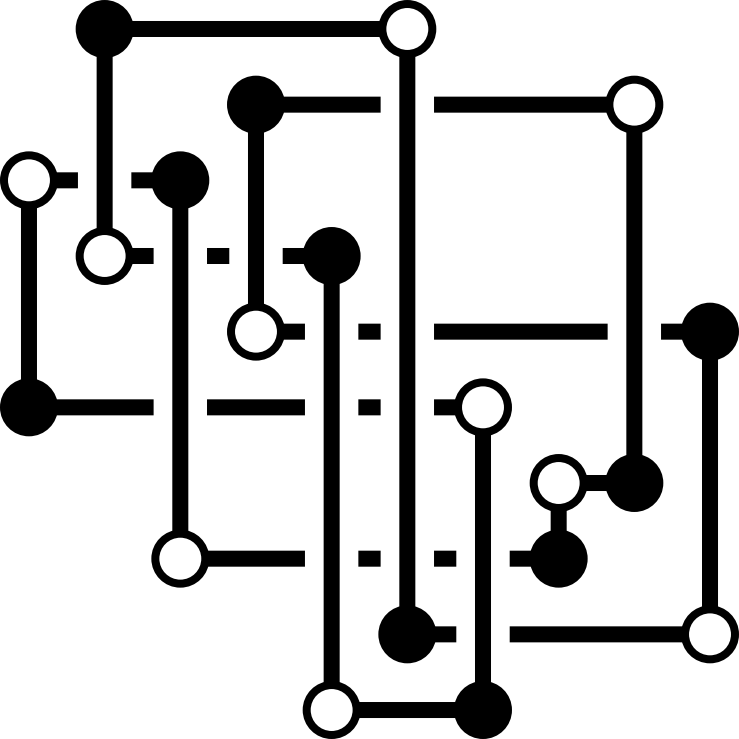



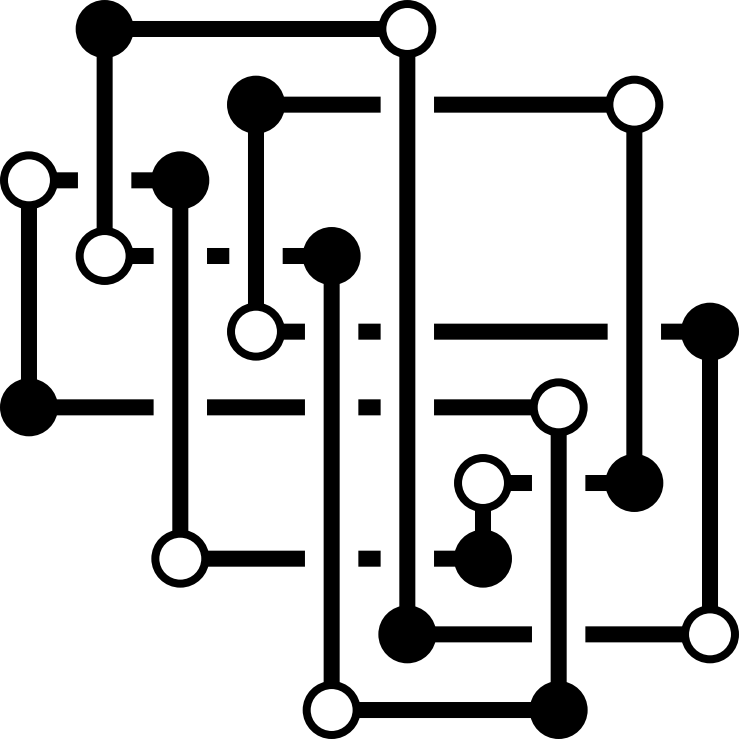

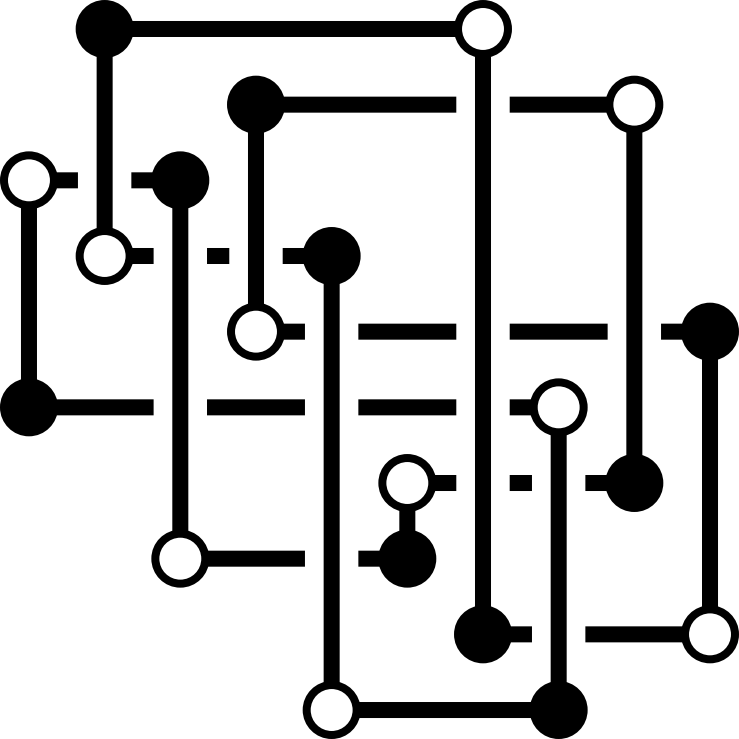

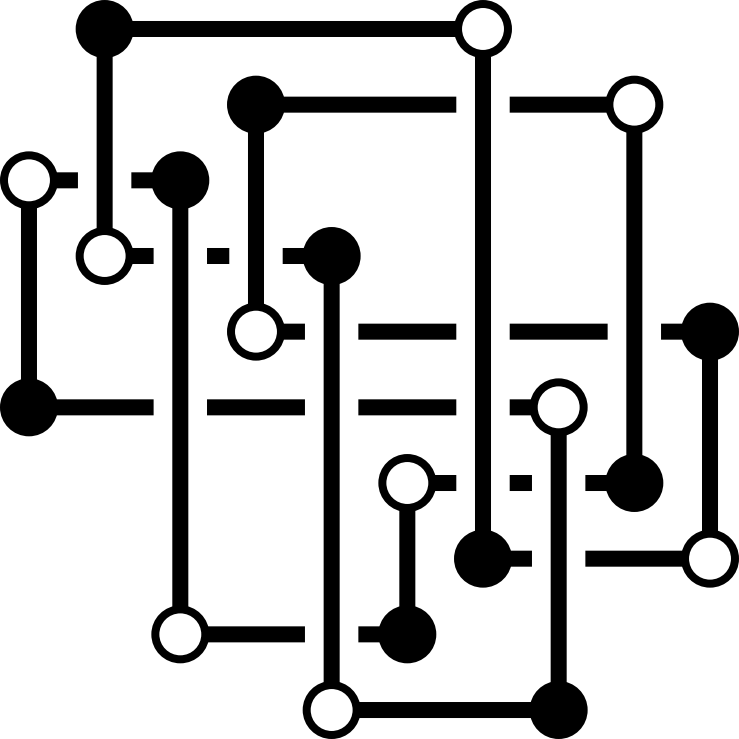

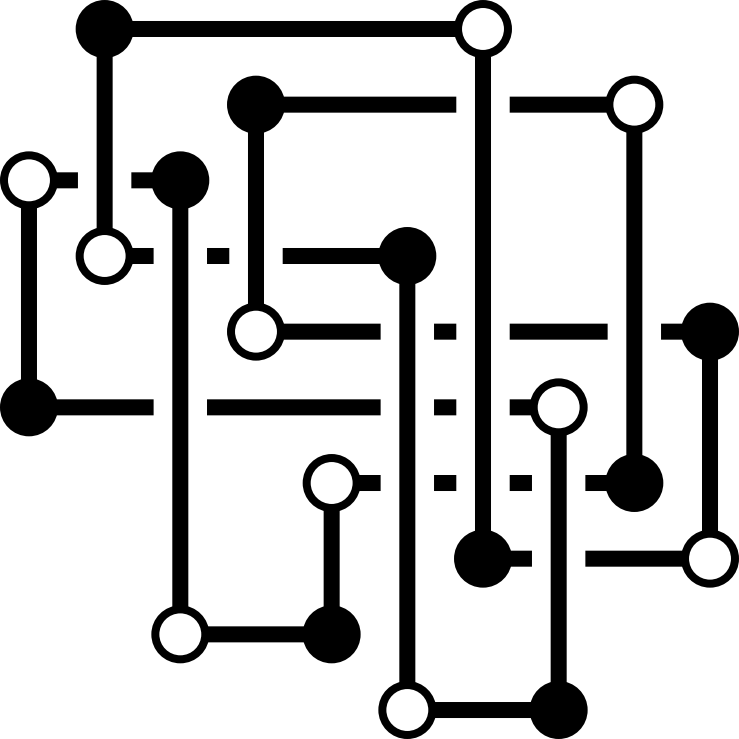

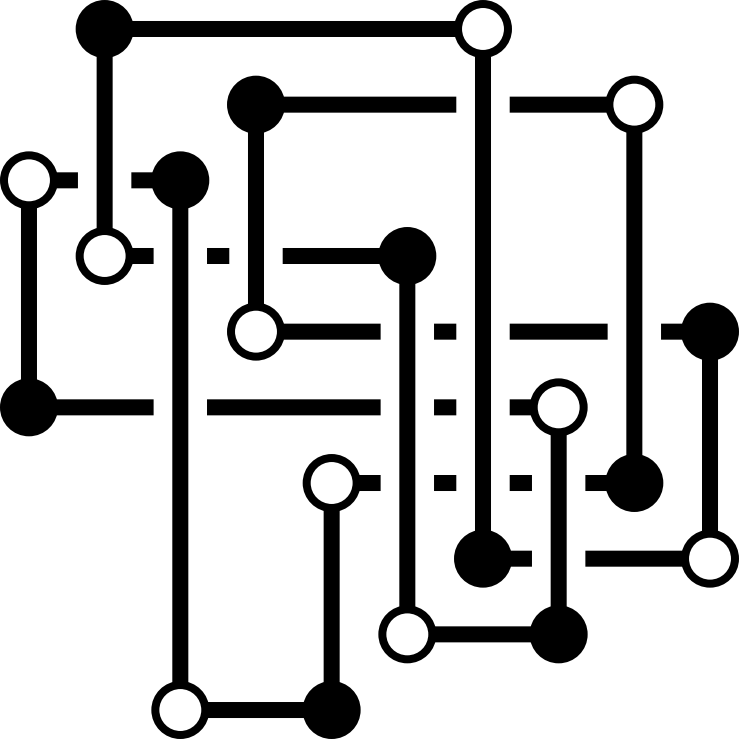

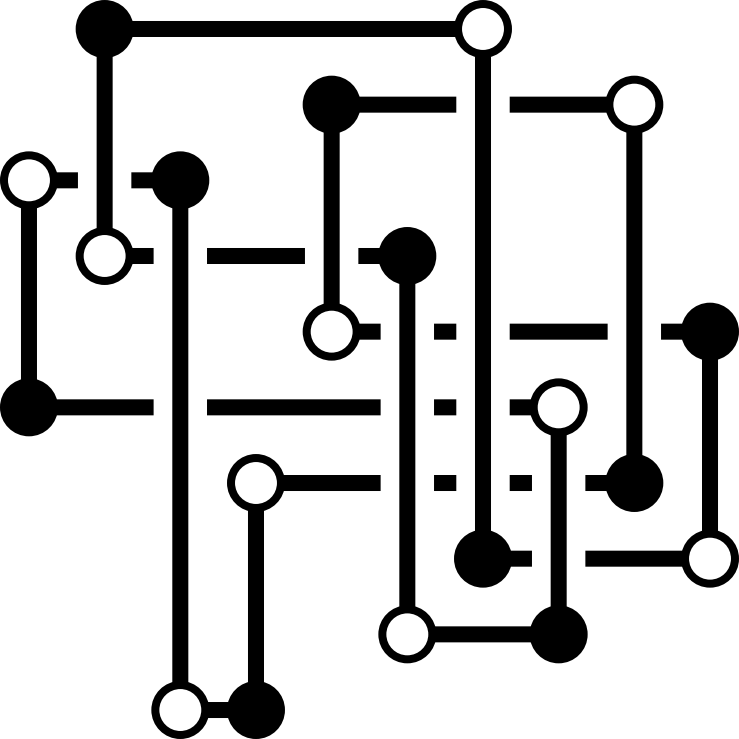

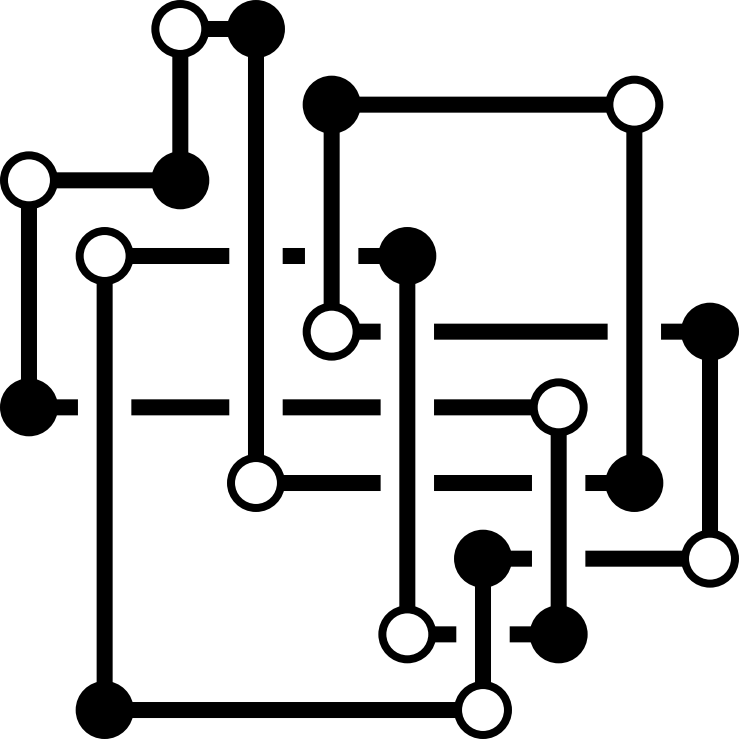

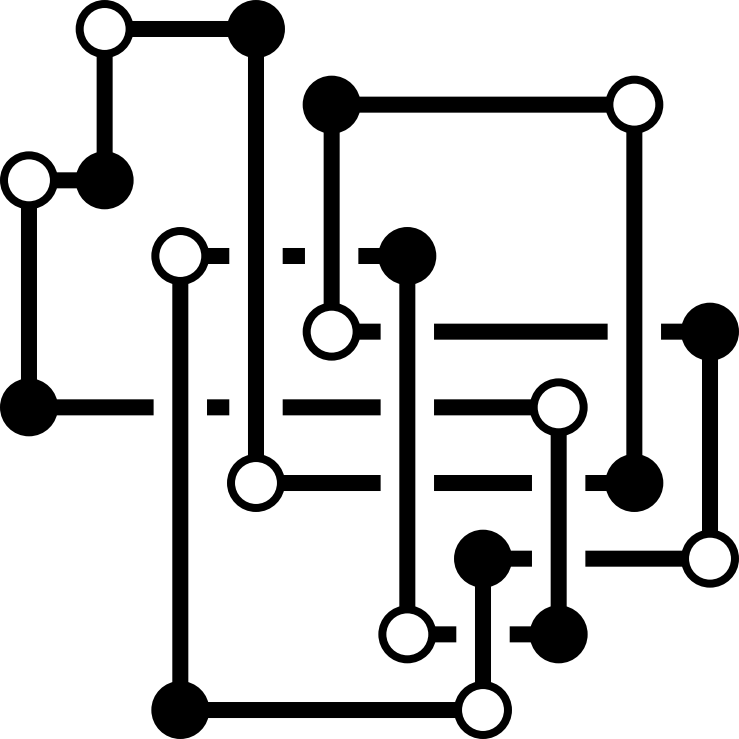



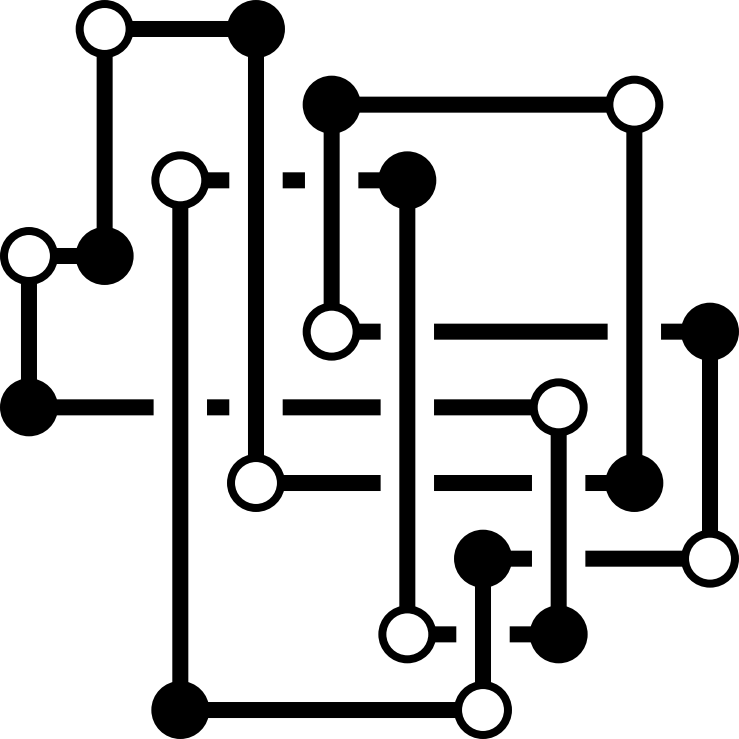

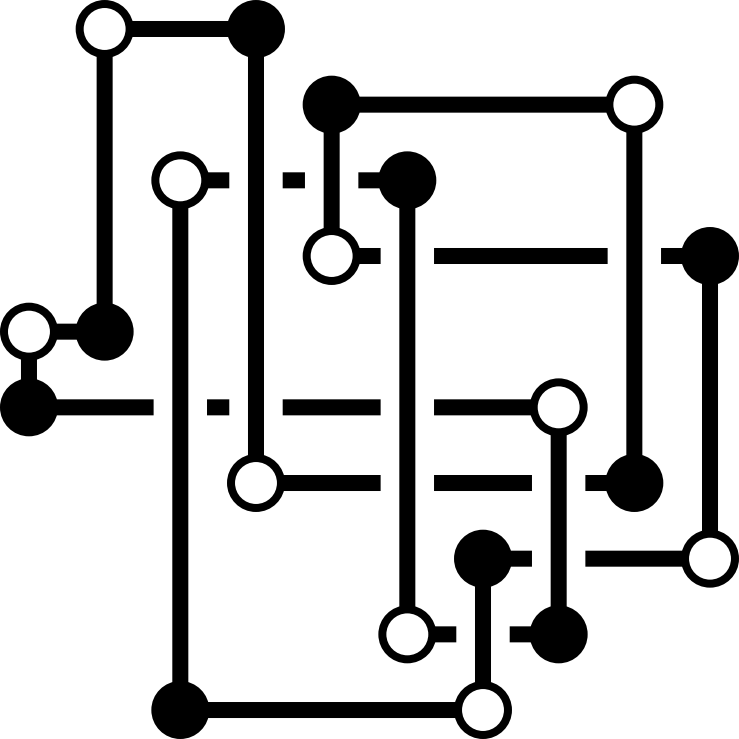

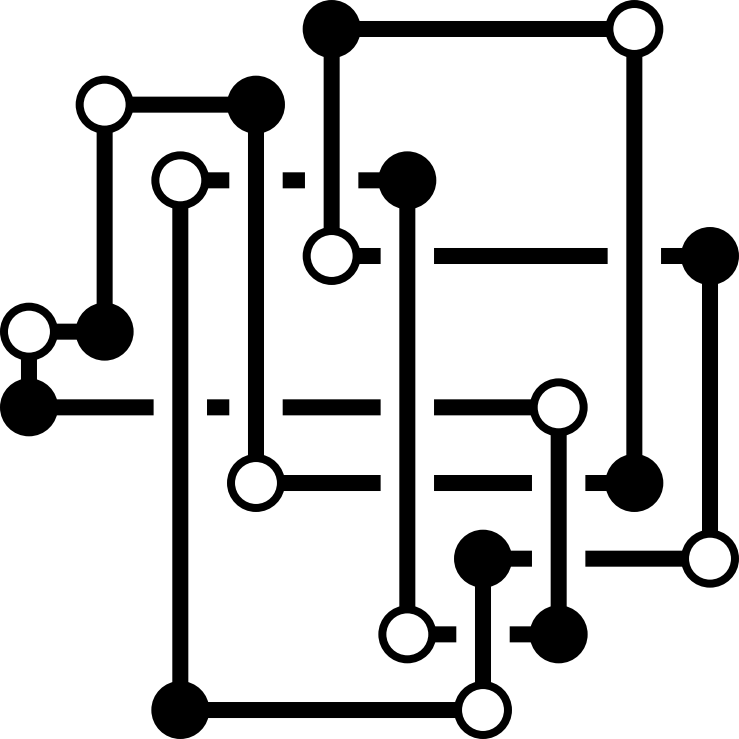

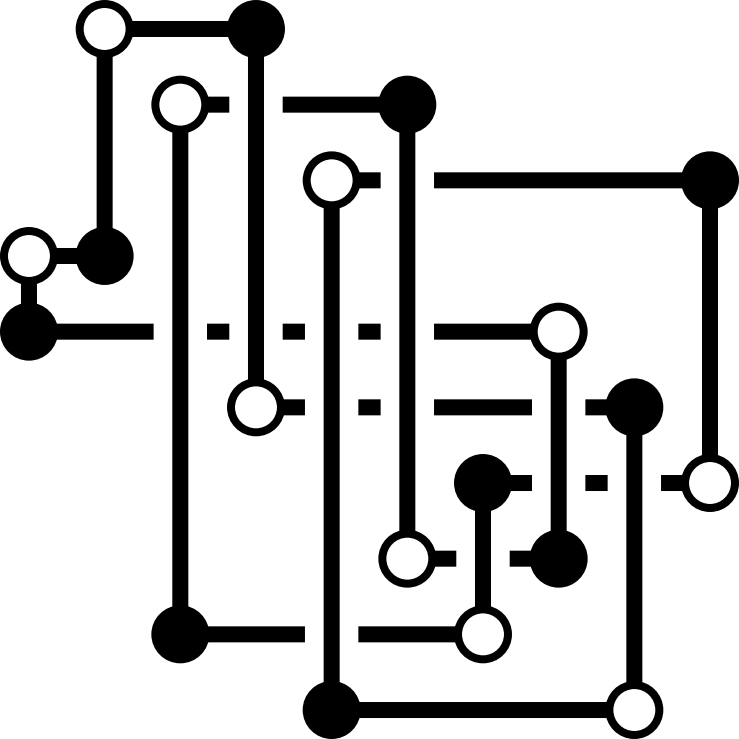

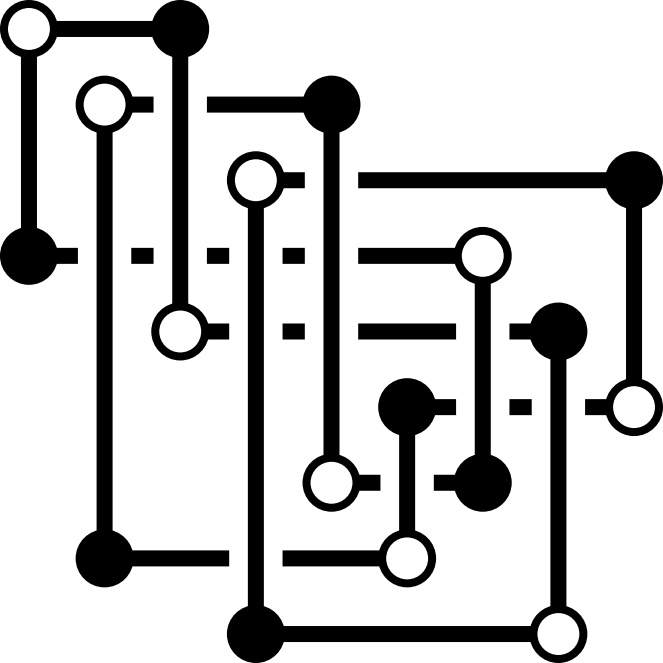

Supplement: Supplementary file 6 [file 9_48-1to3.pdf]
